# Supplementary material for: On the Metrics for Evaluating Monocular Depth Estimation
Source: arXiv:2302.10007 source file (2023-02-20)
Supplement: Supplementary file 1 [file suppl_material.tex]

\section{Evaluation of sampling methods}

In order to bound the number of experiments on 3D object detection, we have started by selecting the best performing method for sampling depth maps and so generating 3D point clouds from images. In Section 3.1 in main paper, % \Sect{produce_pseudo_lidar} 
we described two alternatives. One consists in using all the pixels of the generated depth map for obtaining the corresponding Pseudo-LiDAR, which we called $\pl$. The other consists in using a LiDAR-inspired sampling to obtain the Pseudo-LiDAR, which we called $\pls$. Since we have seen that by working at high resolution we obtain the best depth estimation results (\Tab{mde_in_kitti_3dob_validation}), we focus on this setting to select the sampling method. Moreover, we select two MDE models to bound the number of experiments, namely, AdaBins and MonoDELSNet-SfM. The former is trained with LiDAR supervision (\Tab{mde_approach_comparison}) and is one of the two top-performing methods in depth estimation using high resolution (\Tab{mde_in_kitti_3dob_validation}), while the later also uses SfM self-supervision (\Tab{mde_approach_comparison}) and is the top-performing MDE among those using SfM (\Tab{mde_in_kitti_3dob_validation}). To detect objects, we consider the three approaches introduced in Section 3.3, % \Sect{train_3d_object_detection}, 
{\ie}, Point R-CNN, Voxel R-CNN, and CenterPoint. \Tab{sampling_depth_maps} summarizes the results for their common class (car). We can see clearly that the LiDAR-inspired sampling gives rise to significantly better performing object detectors, particularly, when using voxel-based representations as is the case of Voxel R-CNN and CenterPoint. 

\newcommand{\plsubpls}{\mb{$\pls - \pl$}}
\begin{table}
    \centering
    \scriptsize
    \caption{3D car detection results ($AP_{BEV}, AP_{3D}$) by using different strategies for sampling depth maps, as well as different 3D object detectors (Point R-CNN, Voxel R-CNN, CenterPoint). The sampling is applied to depth maps obtained from MDE models (AdaBins, MonoDELNet-SfM). $\pl$ stands for Pseudo-LiDAR obtained by using all the pixels of the corresponding depth maps, while $\pls$ stands for Pseudo-LiDAR obtained by applying a LiDAR-inspired sampling to the same depth maps (Figure 2 (in main paper), with $\numofbeam=64$). L stands for LiDAR point clouds, thus, for the three detectors this setting produces upper-bound results. These LiDAR point clouds have a one-to-one correspondence with the RGB images used to generate the depth maps with the MDE models. Thus, after sampling these maps, the 3D BBs used with L as object supervision, can be also used with $\pl$ and $\pls$. The images used to generate the depth maps (and so $\pl$ and $\pls$) are from the training set of the Chen {\etal} \cite{Chen:2015} split. The LiDAR training data for the setting L is from the same training set. In all cases, the validation is performed on the validation set of this split.}
    \label{tab:sampling_depth_maps}
    \begin{tabular}{p{1cm}c*{6}{p{0.50cm}}}\Xhline{4\arrayrulewidth} \rowspace
        \centering
        & & \multicolumn{3}{c}{$AP_{BEV}$}&\multicolumn{3}{c}{$AP_{3D}$}\\ \Xhline{2\arrayrulewidth} \rowspace
        {Model}	& {input}	&	{easy}	& {\B mod.} &	{hard}	&	{easy}	& {\B mod.} &	{hard}      \\ \Xhline{4\arrayrulewidth} \rowspace  \baseexpcolor
    % \begin{tabular}{l*{7}{c}}\Xhline{4\arrayrulewidth}
    %     \mb[2em]{}&\mb[1em]{}&\multicolumn{3}{c}{$AP_{BEV}$}&\multicolumn{3}{c}{$AP_{3D}$} \\\hline
    %     \mb[2em]{Model}&\mb[1em]{Input}&\mb[\emvalobsc]{easy}&\mb[\emvalobsc]{\B mod.}&\mb[\emvalobsc]{hard}&\mb[\emvalobsc]{easy}&\mb[\emvalobsc]{\B mod.}&\mb[\emvalobsc]{hard}   \\  \Xhline{4\arrayrulewidth} \rowspace 
        \multicolumn{8}{c}{Point R-CNN} \\ \Xhline{2\arrayrulewidth}  \baseexpcolor
                    &   $\lidar$    &   90.63   &   89.55   &   89.35   &   90.62   &   89.51   &   89.28       \\ \hline \rowspace
                    &   $\pl$       &   65.33   &   41.16   &   33.42   &   61.03   &   39.50   &   32.27       \\ \rowspace 
        AdaBins     &   $\pls$      &   70.86   &   48.31   &   41.12   &   65.66   &   45.98   &   39.56       \\ \rowspace \rowcolor{Red!20}
        Difference  &  \plsubpls    &\UP{05.53} & \UP{07.15}& \UP{07.70}& \UP{04.63}& \UP{06.48}& \UP{07.29}    \\  \rowspace
                    &   $\pl$       &   67.87   &   48.68   &   40.72   &   66.21   &   46.26   &   38.71       \\ \rowspace 
        \mb{MDELS-SfM}&  $\pls$     &   75.58   &   56.07  &  48.68     &   71.15   &   53.31  &    45.92       \\ \rowspace \rowcolor{Red!20}
        Difference  &  \plsubpls    &\UP{07.71} & \UP{07.39}& \UP{07.96}& \UP{04.94}& \UP{07.05}& \UP{07.21}    \\ \rowspace
        \Xhline{4\arrayrulewidth} \rowspace 
        \multicolumn{8}{c}{Voxel R-CNN} \\ \Xhline{2\arrayrulewidth}  \baseexpcolor
                    &   $\lidar$    &   97.33   &   89.71   &   89.35   &   97.29   &   89.70   &   89.33       \\ \hline \rowspace
                    &   $\pl$       &   20.22   &   14.13   &   13.22   &   18.07   &   12.72   &   11.21       \\ \rowspace
        AdaBins     &   $\pls$      &   70.77   &   52.34   &   46.46   &   66.18   &   47.44   &   43.90       \\ \rowspace \rowcolor{Red!20}
        Difference  &  \plsubpls    & \UP{50.55}& \UP{38.21}& \UP{33.24}& \UP{48.11}& \UP{34.72}& \UP{32.69}    \\ \rowspace
                    &   $\pl$       &   12.18   &   08.72   &   08.10   &   09.15   &   07.19   &   06.47       \\ \rowspace
        \mb{MDELS-SfM}&  $\pls$     &   74.91   &   56.07   &   53.17   &   71.51   &   53.11   &   47.06       \\ \rowspace \rowcolor{Red!20}
        Difference  &  \plsubpls    & \UP{63.72}& \UP{48.67}& \UP{46.13}& \UP{64.82}& \UP{48.45}& \UP{42.26}    \\ \rowspace \Xhline{4\arrayrulewidth} \rowspace 
        \multicolumn{8}{c}{CenterPoint} \\ \Xhline{2\arrayrulewidth}  \baseexpcolor
                    &   $\lidar$    &   95.25   &   89.88   &   89.30   &   95.17   &   89.85   &   89.21       \\ \hline \rowspace
                    &   $\pl$       &   11.21   &   09.09   &   09.09   &   09.91   &   09.09   &   09.09       \\ \rowspace
        AdaBins     &   $\pls$      &   67.92   &   47.21   &   43.04   &   63.62   &   44.85   &   38.63       \\  \rowspace \rowcolor{Red!20}
        Difference  &  \plsubpls    & \UP{56.71}& \UP{38.12}& \UP{33.95}& \UP{53.71}& \UP{35.76}& \UP{29.54}    \\  \rowspace
                    &   $\pl$       &   10.74   &   09.81   &   09.09   &   10.06   &   09.09   &   09.09       \\ \rowspace
        \mb{MDELS-SfM}&  $\pls$     &   69.23   &   52.87   &   46.46   &   63.60   &   48.56   &   43.29       \\  \rowspace \rowcolor{Red!20}
        Difference  &  \plsubpls    & \UP{58.49}& \UP{43.06}& \UP{37.37}& \UP{53.54}& \UP{39.47}& \UP{34.20}    \\ \rowspace
        \Xhline{4\arrayrulewidth}
    \end{tabular}
\end{table}

\section{Depth Estimation quantitative results on validation set \cite{Chen:2015}}

An additional detail to take into account concerns image resolution, which turns out not to be equal for all images of the KITTI dataset. We can find differences of $\sim6$ pixels in the number of rows, and $\si22$ pixels in the number of columns. The LiDAR-based depth maps (ground truth) are generated to have the same resolution as their associated images. This fact together with the differences among the CNN architectures for depth estimation have provoked differences on the working resolution of the depth estimation models. In order to clarify this, we must consider \Tab{mde_approach_comparison}. We see that all the models except AdaBins are prepared to work on two resolutions, namely, high and low. The high one varies a bit from model to model. The low one is the same for all models and has been the standard one used in the literature to research on MDE. Since the resolution of KITTI original images runs on $[1224 - 1242]\times[370 - 376]$ pixels, working with both high and low resolution involves resizing the KITTI images ({\eg}, using LANCZOS interpolation) for training and inference. For the high resolution, the resizing is relatively small, for the low resolution there is a strong down-scaling. 

For evaluating the depth estimation results (using abs-rel, rms, {\etc}), no matter the working resolution of the depth estimation models, nearest neighbourhood is applied to compare each estimated depth with the ground truth. As we have mentioned before, for each KITTI image its LiDAR-based depth map (ground truth) has the same resolution. Thus, these ground truth maps are of higher resolution than the estimated ones, specially in case of using the low resolution setting. On the other hand, for generating Pseudo-LiDAR, the estimated depth maps are resized to the resolution of the original KITTI images using nearest neighbourhood too. Again, when working at high resolution, this resizing is relatively small, while for low resolution this implies a more significant up-scaling. Finally, AdaBins handles the images of KITTI at their original resolution at training and inference times. 

Comparing resolutions, we see that the higher the resolution the better the performance of the same models. For both resolutions MonoDELSNet-SfM outperforms MonoDEVSNet-SfM. 
In fact, in the standard resolution, ADtDBR is the best performing model. At the higher resolution, it still  

\begin{table}
    \centering
    \scriptsize
    \caption{\textit{\IL{Lower Resolution}}: Absolute depth results (up to $80$m) for the images of the validation set of the Chen {\etal} \cite{Chen:2015} split. We use the models trained by the corresponding authors for PackNet, MonoDepth2, and AdaBins, the rest are trained by us. All the models are based on the same training and validation sets. SDNet must be considered an upper-bound since it uses a stereo pair at testing time, while all the other models work on single images. Bold stands for \textbf{best} and underline for \IL{second best}.}
    \label{tab:mde_in_kitti_3dob_validation} 
    \begin{tabular}{|p{1.6cm}*{7}{p{0.45cm}}|} \Xhline{4\arrayrulewidth}  \rowspace
        {\textbf{Model}}&{\mb{\textbf{abs-rel}}}&{\mb{\textbf{sq-rel}}}&{\textbf{rms}}&{\mb{\textbf{rms-log}}}&{\bm{$1.25$}}&{\bm{$1.25^2$}}&{\bm{$1.25^3$}}\\ \Xhline{4\arrayrulewidth} \rowspace
        \multicolumn{8}{c}{Low (standard) resolution (see \Tab{mde_approach_comparison})} \\ \Xhline{3\arrayrulewidth} \rowspace
        PackNet-SfM	    &   0.103   &   0.804   &   4.780   &   0.198   &   0.882   &   0.954   &   0.977       \\ \hline \rowspace
        MD2-St          &   0.097   &   0.852   &   4.919   &   0.205   &   0.875   &   0.948   &   0.974       \\ \hline \rowspace
        MD2-St+SfM      &   0.096   &   0.795   &   4.746   &   0.192   &   0.885   &   0.957   &   0.978       \\ \hline \rowspace
        MDEVS-SfM       &   0.094   &   0.660   &   4.297   &   0.180   &\IL{0.896} &\IL{0.964} &   0.982       \\ \hline \rowspace
        MDELS-SfM       &\IL{0.082} &\IL{0.535} &\IL{3.915} &\IL{0.169} & \B0.910   & \B0.966   &\IL{0.983}     \\ \hline \rowspace
        ADtDBR	    & \B0.079   & \B0.527   & \B3.900   & \B0.167   & \B0.910   & \B0.966   & \B0.984       \\ \Xhline{3\arrayrulewidth}
        % \multicolumn{8}{c}{High resolution (see \Tab{mde_approach_comparison})} \\ \Xhline{3\arrayrulewidth} \rowspace
        % PackNet-SfM	    &   0.101   &   0.901   &   4.774   &   0.199   &   0.888   &   0.955   &   0.972       \\ \hline \rowspace
        % MD2-St          &   0.096   &   0.788   &   4.719   &   0.198   &   0.883   &   0.952   &   0.976       \\ \hline \rowspace
        % MD2-St+SfM      &   0.095   &   0.769   &   4.609   &   0.188   &   0.892   &   0.959   &   0.979       \\ \hline \rowspace
        % MDEVS-SfM       &   0.090   &   0.617   &   4.107   &   0.177   &   0.903   &   0.966   &   0.982       \\ \hline \rowspace
        % MDELS-SfM       & \IL{0.077}& \IL{0.511}&   3.837   &   0.172   &   0.911   &   0.966   &   0.982       \\ \hline \rowspace
        % ADtDBR	    & \B0.073   & \B0.495   & \B3.761   & \IL{0.166}& \IL{0.918}& \IL{0.967}& \IL{0.983}    \\ \hline \rowspace
        % \mb{MDELS-SfM/RN}&   0.079   &   0.537   &   3.904   &   0.171   &   0.909   &   0.966   &   0.982       \\ \hline \rowspace
        % AdaBins	        &   0.080   &   0.512   & \IL{3.821}& \B0.164   & \B0.920   & \B0.969   & \B0.984       \\ \Xhline{2\arrayrulewidth} \rowspace
        % SDNet           &  \B0.044  &  \B0.365  &  \B3.050  &  \B0.136  &  \B0.962  &  \B0.978  &  \B0.987      \\ \Xhline{4\arrayrulewidth}
    \end{tabular}
\end{table}

\section{3D-Object detection results (Point R-CNN, Voxel R-CNN and CenterPoint).}

\begin{table}
    \centering
    \scriptsize
    \caption{{\textit{\IL{Lower Resolution}}}: Results on 3D car detection ($AP_{BEV}, AP_{3D}$) using Point R-CNN, Voxel R-CNN and CenterPoint. We complement these results with two depth estimation metrics (abs-rel, rms). Taking \Fig{experiment-protocol} as reference, $AP_{BEV}$ and $AP_{3D}$ play the role of Eval 3D-OD, while abs-rel and rms are part of Eval DE. LiDAR PC refers to training with actual raw LiDAR 3D point clouds, and SDNet estimates depth from stereo images. Thus, these two methods can be seen as upper-bounds for the rest, which generate the corresponding 3D point clouds after performing MDE. Focusing on the MDE models, bold stands for \textbf{best} and underline for \IL{second best} within each 3d object detector block.}
    \label{tab:SOTA_KITTI_3dobject_bev_3d} 
    \hskip-0.15cm
    \begin{tabular}{p{1.5cm}*{8}{p{0.40cm}}}\Xhline{4\arrayrulewidth} \rowspace
        &\multicolumn{3}{c}{$AP_{BEV}$}&\multicolumn{3}{c}{$AP_{3D}$}&\multicolumn{2}{c}{DE}\\ \Xhline{2\arrayrulewidth} \rowspace
        {Model}		&	{easy}	& {\B mod.} &	{hard}	&	{easy}	& {\B mod.} &	{hard} 	&\mb{abs-rel} & {rms} \\ \Xhline{4\arrayrulewidth} \rowspace      
        \multicolumn{9}{c}{Point R-CNN} \\ \Xhline{2\arrayrulewidth} \rowspace \baseexpcolor
        LiDAR PC    &   90.63   &   89.55   &   89.35   &   90.62   &   89.51   &   89.28   &   -       &   -              \\ \Xhline{3\arrayrulewidth} \rowspace
        % \multicolumn{9}{c}{Low resolution (see \Tab{mde_approach_comparison})} \\ \Xhline{3\arrayrulewidth} \rowspace
        PackNet-SfM	&   43.27   &   28.93   &   24.20   &   39.48   &   26.92   &   23.17   &   0.103   &   4.780   \\ \hline \rowspace
        MD2-St      &   59.48   &   38.93   &   32.08   &   54.37   &   36.28   &   30.94   &   0.097   &   4.919   \\ \hline \rowspace
        MD2-St+SfM  &   54.97   &   35.84   &   30.77   &   51.09   &   31.55   &   27.69   &   0.096   &   4.746   \\ \hline \rowspace
        MDEVS-SfM   &   64.36   &   44.30   &   38.86   &   60.00   &   39.54   &   36.22   &   0.094   &   4.297   \\ \hline \rowspace
        MDELS-SfM	& \IL{65.43}& \IL{47.01}& \IL{39.82}& \IL{62.08}& \IL{43.61}& \IL{37.94}& \IL{0.082}& \IL{3.915}\\ \hline \rowspace
        ADtDBR	& \B66.23   & \B47.24   & \B40.13   & \B63.85   & \B44.42   & \B38.31   & \B0.079   & \B3.900   \\ \hline \Xhline{4\arrayrulewidth} \rowspace
        \multicolumn{9}{c}{Voxel R-CNN} \\ \Xhline{2\arrayrulewidth} \rowspace \baseexpcolor
        LiDAR PC    &   97.33   &   89.71   &   89.35   &   97.29   &   89.70   &   89.33   &   -       &   -              \\ \Xhline{3\arrayrulewidth} \rowspace
        % \multicolumn{9}{c}{Low resolution (see \Tab{mde_approach_comparison})} \\ \Xhline{3\arrayrulewidth} \rowspace
        Packnet-SfM	&   48.11   &   33.71   &   29.27   &   42.31   &   29.68   &   26.97   &   0.103   &   4.780   \\ \hline \rowspace
        MD2-St      &   59.17   &   41.88   &   36.32   &   54.85   &   37.38   &   34.01   &   0.097   &   4.919   \\ \hline \rowspace
        MD2-St+SfM  &   56.12   &   37.27   &   34.52   &   53.01   &   34.60   &   29.74   &   0.096   &   4.746   \\ \hline \rowspace
        MDEVS-SfM   &   63.96   &   45.08   &   42.62   &   60.42   &   42.47   &   37.51   &   0.094   &   4.297   \\ \hline \rowspace
        MDELS-SfM   & \IL{65.04}& \IL{46.85}& \IL{43.62}& \IL{62.22}& \IL{44.68}& \IL{38.72}& \IL{0.082}& \IL{3.915}\\ \hline \rowspace
        ADtDBR	& \B69.32   & \B47.77   & \B44.80   & \B64.20   & \B45.67   & \B42.40   & \B0.079   & \B3.900   \\ \hline \Xhline{4\arrayrulewidth} \rowspace
        \multicolumn{9}{c}{CenterPoint} \\ \Xhline{2\arrayrulewidth} \rowspace \baseexpcolor
        LiDAR PC    &   95.25   &   89.88   &   89.30   &   95.17   &   89.85   &   89.21   &      -    &   -  \\ \Xhline{3\arrayrulewidth} \rowspace
        % \multicolumn{9}{c}{Low resolution (see \Tab{mde_approach_comparison})} \\ \Xhline{3\arrayrulewidth} \rowspace        
        PackNet-SfM	    &   42.34   &   29.74   &   25.92   &   36.55   &   26.09   &   23.25   &   0.103   &   4.780       \\ \hline \rowspace
        MD2-St          &   56.50   &   39.79   &   34.97   &   52.63   &   35.92   &   31.93   &   0.097   &   4.919       \\ \hline \rowspace
        MD2-St+SfM      &   54.00   &   35.49   &   32.01   &   50.29   &   32.32   &   28.31   &   0.096   &   4.746       \\ \hline \rowspace
        MDEVS-SfM       &   57.46   &   40.86   &   36.28   &   51.71   &   38.02   &   33.85   &   0.094   &   4.297       \\ \hline \rowspace
        MDELS-SfM	    &   62.48   & \B45.61   & \IL{40.99}& \IL{56.97}& \IL{42.25}& \IL{37.14}& \IL{0.082}& \IL{3.915}    \\ \hline \rowspace  
        ADtDBR	    & \B62.75   & \IL{45.38}& \B41.23   & \B58.80   & \B42.69   & \B37.36   & \B0.079   & \B3.900       \\ \hline \Xhline{4\arrayrulewidth} \rowspace
    \end{tabular}
\end{table}

\begin{table}
    \centering
    \scriptsize
    \caption{Results on 3D car detection ($AP_{BEV}, AP_{3D}$) using Point R-CNN. We complement these results with two depth estimation metrics (abs-rel, rms). Taking \Fig{experiment-protocol} as reference, $AP_{BEV}$ and $AP_{3D}$ play the role of Eval 3D-OD, while abs-rel and rms are part of Eval DE. LiDAR PC refers to training with actual LiDAR 3D point clouds, and SDNet estimates depth from stereo images. Thus, these two methods can be seen as upper-bounds for the rest, which generate the corresponding 3D point clouds after performing MDE. Focusing on the MDE models, bold stands for \textbf{best} and underline for \IL{second best} within each resolution block.}
    \label{tab:SOTA_KITTI_3dobject_bev_3d_point_rcnn} 
    \hskip-0.15cm
    \begin{tabular}{p{1.5cm}*{8}{p{0.40cm}}}\Xhline{4\arrayrulewidth} \rowspace
        &\multicolumn{3}{c}{$AP_{BEV}$}&\multicolumn{3}{c}{$AP_{3D}$}&\multicolumn{2}{c}{DE}\\ \Xhline{2\arrayrulewidth} \rowspace
        {Model}		&	{easy}	& {\B mod.} &	{hard}	&	{easy}	& {\B mod.} &	{hard} 	&\mb{abs-rel} & {rms}       \\ \Xhline{4\arrayrulewidth} \rowspace  \baseexpcolor      
        LiDAR PC &   90.63   &   89.55   &   89.35   &   90.62   &   89.51   &   89.28   &   -       &   -              \\ \Xhline{3\arrayrulewidth} \rowspace
        % standard resolution
        \multicolumn{9}{c}{Low resolution (see \Tab{mde_approach_comparison})} \\ \Xhline{3\arrayrulewidth} \rowspace
        PackNet-SfM	    &   43.27   &   28.93   &   24.20   &   39.48   &   26.92   &   23.17   &   0.103   &   4.780   \\ \hline \rowspace
        MD2-St          &   59.48   &   38.93   &   32.08   &   54.37   &   36.28   &   30.94   &   0.097   &   4.919   \\ \hline \rowspace
        MD2-St+SfM      &   54.97   &   35.84   &   30.77   &   51.09   &   31.55   &   27.69   &   0.096   &   4.746   \\ \hline \rowspace
        MDEVS-SfM       &   64.36   &   44.30   &   38.86   &   60.00   &   39.54   &   36.22   &   0.094   &   4.297   \\ \hline \rowspace
        MDELS-SfM	    & \IL{65.43}& \IL{47.01}& \IL{39.82}& \IL{62.08}& \IL{43.61}& \IL{37.94}& \IL{0.082}& \IL{3.915}\\ \hline \rowspace
        ADtDBR	    & \B66.23   & \B47.24   & \B40.13   & \B63.85   & \B44.42   & \B38.31   & \B0.079   & \B3.900   \\ \hline \Xhline{4\arrayrulewidth} \rowspace
        % High resolution
        \multicolumn{9}{c}{High resolution (see \Tab{mde_approach_comparison})} \\ \Xhline{3\arrayrulewidth} \rowspace
        PackNet-SfM	    &   47.86   &   32.53   &   30.50   &   45.74   &   31.39   &   27.84   &   0.101   &   4.774   \\ \hline \rowspace
        MD2-St          &   64.34   &   40.88   &   37.21   &   59.96   &   39.36   &   32.41   &   0.096   &   4.719   \\ \hline \rowspace
        MD2-St+SfM      &   58.81   &   37.68   &   31.63   &   53.14   &   35.37   &   30.10   &   0.095   &   4.609   \\ \hline \rowspace
        MDEVS-SfM	    &   66.17   &   47.66   &   45.30   &   64.33   &   45.93   &   40.01   &   0.090   &   4.107   \\ \hline \rowspace
        MDELS-SfM	    & \B75.58   & \B56.07   & \B48.68   & \B71.15   & \B53.31   & \B45.92   & \IL{0.077}&   3.837   \\ \hline \rowspace
        ADtDBR        & \IL{74.57}& \IL{54.35}& \IL{47.25}& \IL{68.13}& \IL{47.42}& \IL{42.84}& \B0.073   & \B3.761   \\ \hline \rowspace
        \mb{MDELS-SfM/RN}&   70.50   &   48.97   &   45.41   &   64.89   &   47.15   &   39.87   &   0.079   &   3.904  \\ \hline \rowspace
        AdaBins	        &   70.86   &   48.31   &   41.12   &   65.66   &   45.98   &   39.56   &   0.080   & \IL{3.821}\\ \Xhline{2\arrayrulewidth} \rowspace   \baseexpcolor
        SDNet	        &   89.79   &   77.98   &   69.62   &   89.59   &   75.61   &   67.36   &   0.044   &   3.050   \\ \hline \Xhline{4\arrayrulewidth}
        \end{tabular}
\end{table}

\begin{table}
    \centering
    \scriptsize
    \caption{Analogous to \Tab{SOTA_KITTI_3dobject_bev_3d_point_rcnn} but using Voxel R-CNN.}
    \label{tab:SOTA_KITTI_3dobject_bev_3d_voxel_rcnn} 
    \hskip-0.15cm
    \begin{tabular}{p{1.5cm}*{8}{p{0.40cm}}}\Xhline{4\arrayrulewidth} \rowspace
        &\multicolumn{3}{c}{$AP_{BEV}$}&\multicolumn{3}{c}{$AP_{3D}$}&\multicolumn{2}{c}{DE}\\ \Xhline{2\arrayrulewidth} \rowspace
        {Model}		&	{easy}	& {\B mod.} &	{hard}	&	{easy}	& {\B mod.} &	{hard} 	&\mb{abs-rel} & {rms}       \\ \Xhline{4\arrayrulewidth} \rowspace  \baseexpcolor      
        LiDAR PC &   97.33   &   89.71   &   89.35   &   97.29   &   89.70   &   89.33   &   -       &   -              \\ \Xhline{3\arrayrulewidth} \rowspace
        % standard resolution
        \multicolumn{9}{c}{Low resolution (see \Tab{mde_approach_comparison})} \\ \Xhline{3\arrayrulewidth} \rowspace
        Packnet-SfM	    &   48.11   &   33.71   &   29.27   &   42.31   &   29.68   &   26.97   &   0.103   &   4.780   \\ \hline \rowspace
        MD2-St          &   59.17   &   41.88   &   36.32   &   54.85   &   37.38   &   34.01   &   0.097   &   4.919   \\ \hline \rowspace
        MD2-St+SfM      &   56.12   &   37.27   &   34.52   &   53.01   &   34.60   &   29.74   &   0.096   &   4.746   \\ \hline \rowspace
        MDEVS-SfM       &   63.96   &   45.08   &   42.62   &   60.42   &   42.47   &   37.51   &   0.094   &   4.297   \\ \hline \rowspace
        MDELS-SfM       & \IL{65.04}& \IL{46.85}& \IL{43.62}& \IL{62.22}& \IL{44.68}& \IL{38.72}& \IL{0.082}& \IL{3.915}\\ \hline \rowspace
        ADtDBR	    & \B69.32   & \B47.77   & \B44.80   & \B64.20   & \B45.67   & \B42.40   & \B0.079   & \B3.900   \\ \hline \Xhline{4\arrayrulewidth} \rowspace
        % High resolution
        \multicolumn{9}{c}{High resolution (see \Tab{mde_approach_comparison})} \\ \Xhline{3\arrayrulewidth} \rowspace
        PackNet-SfM	    &   55.23   &   37.12   &   35.80   &   52.19   &   34.71   &   33.86   &   0.101   &   4.774   \\ \hline \rowspace
        MD2-St          &   65.21   &   45.74   &   42.64   &   62.21   &   42.54   &   37.47   &   0.096   &   4.719   \\ \hline \rowspace
        MD2-St+SfM      &   57.98   &   37.72   &   35.09   &   52.87   &   35.40   &   30.54   &   0.095   &   4.609   \\ \hline \rowspace
        MDEVS-SfM	    &   65.73   &   46.90   &   45.24   &   63.06   &   44.69   &   42.84   &   0.090   &   4.107   \\ \hline \rowspace
        MDELS-SfM	    & \IL{74.91}& \IL{56.07}& \IL{53.17}& \IL{71.51}& \IL{53.11}& \IL{47.06}& \IL{0.077}&   3.837   \\ \hline \rowspace
        ADtDBR        & \B75.90   & \B57.39   & \B54.23   & \B73.97   & \B55.64   & \B48.73   & \B0.073   & \B3.761   \\ \hline \rowspace
        \mb{MDELS-SfM/RN}&   69.94   &   52.59   &   46.62   &   65.42   &   47.68   &   43.87   &   0.079   &   3.904  \\ \hline \rowspace
        AdaBins	        &   70.77   &   52.34   &   46.46   &   66.18   &   47.44   &   43.90   &   0.080   & \IL{3.821}\\ \hline \Xhline{2\arrayrulewidth} \rowspace  \baseexpcolor
        SDNet	        &   90.35   &   79.15   &   76.35   &   90.28   &   78.39   &   70.35   &   0.044   &   3.050   \\ \hline \Xhline{4\arrayrulewidth}
    \end{tabular}
\end{table}

\begin{table}
    \scriptsize
    \caption{Analogous to \Tab{SOTA_KITTI_3dobject_bev_3d_point_rcnn} but using CenterPoint.}
    \label{tab:SOTA_KITTI_3dobject_bev_3d_center_point} 
    \hskip-0.15cm
    \begin{tabular}{p{1.5cm}*{8}{p{0.40cm}}}\Xhline{4\arrayrulewidth} \rowspace
        \centering
        &\multicolumn{3}{c}{$AP_{BEV}$}&\multicolumn{3}{c}{$AP_{3D}$}&\multicolumn{2}{c}{DE}\\ \Xhline{2\arrayrulewidth} \rowspace
        {Model}		&	{easy}	& {\B mod.} &	{hard}	&	{easy}	& {\B mod.} &	{hard} 	&\mb{abs-rel} & {rms}      \\ \Xhline{4\arrayrulewidth} \rowspace  \baseexpcolor      
        LiDAR PC    &   95.25   &   89.88   &   89.30   &   95.17   &   89.85   &   89.21   &      -    &   -  \\ \Xhline{3\arrayrulewidth} \rowspace
        % standard resolution
        \multicolumn{9}{c}{Low resolution (see \Tab{mde_approach_comparison})} \\ \Xhline{3\arrayrulewidth} \rowspace        
        PackNet-SfM	    &   42.34   &   29.74   &   25.92   &   36.55   &   26.09   &   23.25   &   0.103   &   4.780       \\ \hline \rowspace
        MD2-St          &   56.50   &   39.79   &   34.97   &   52.63   &   35.92   &   31.93   &   0.097   &   4.919       \\ \hline \rowspace
        MD2-St+SfM      &   54.00   &   35.49   &   32.01   &   50.29   &   32.32   &   28.31   &   0.096   &   4.746       \\ \hline \rowspace
        MDEVS-SfM       &   57.46   &   40.86   &   36.28   &   51.71   &   38.02   &   33.85   &   0.094   &   4.297       \\ \hline \rowspace
        MDELS-SfM	    &   62.48   & \B45.61   & \IL{40.99}& \IL{56.97}& \IL{42.25}& \IL{37.14}& \IL{0.082}& \IL{3.915}    \\ \hline \rowspace  
        ADtDBR	    & \B62.75   & \IL{45.38}& \B41.23   & \B58.80   & \B42.69   & \B37.36   & \B0.079   & \B3.900       \\ \hline \Xhline{4\arrayrulewidth} \rowspace
        % High resolution
        \multicolumn{9}{c}{High resolution (see \Tab{mde_approach_comparison})} \\ \Xhline{3\arrayrulewidth} \rowspace
        PackNet-SfM	    &   49.89   &   35.10   &   32.10   &   45.44   &   32.33   &   29.10   &   0.101   &   4.774       \\ \hline \rowspace
        MD2-St          &   62.14   &   43.22   &   37.59   &   56.43   &   39.82   &   34.96   &   0.096   &   4.719       \\ \hline \rowspace
        MD2-St+SfM      &   51.00   &   35.12   &   31.72   &   47.01   &   31.50   &   28.12   &   0.095   &   4.609       \\ \hline \rowspace
        MDEVS-SfM	    &   61.13   &   44.63   &   42.16   &   56.66   &   41.63   &   37.10   &   0.090   &   4.107       \\ \hline \rowspace
        MDELS-SfM	    & \IL{69.23}& \IL{52.87}& \IL{46.46}& \IL{63.60}& \IL{48.56}& \IL{43.29}& \IL{0.077}&   3.837       \\ \hline \rowspace
        ADtDBR        & \B74.04   & \B56.14   & \B51.96   & \B68.69   & \B53.58   & \B47.27   & \B0.073   & \B3.761       \\ \hline \rowspace
        \mb{MDELS-SfM/RN}&   66.72   &   49.65   &   44.82   &   62.57   &   45.65   &   41.14   &   0.079   &   3.904       \\ \hline \rowspace
        AdaBins	        &   67.92   &   47.21   &   43.04   &   63.62   &   44.85   &   38.63   &   0.080   & \IL{3.821}    \\ \hline \Xhline{2\arrayrulewidth} \rowspace  \baseexpcolor
        SDNet	        &   89.78   &   77.76   &   73.75   &   89.27   &   75.70   &   68.51   &   0.044   &   3.050       \\ 
        \hline \Xhline{4\arrayrulewidth}
    \end{tabular}
\end{table}

\section{Comparing Rankings}
\Fig{ranking_rms_hr} and \Fig{ranking_rms_sr} are analogous using the rms metric, while \Fig{ranking_a1_hr} is based on $\delta < 1.25$ metric. When working on low resolution, it seems that the correspondence is higher than when working at high resolution. However, high resolution is more interesting since we have seen that the produced Pseudo-LiDAR gives rise to better performing 3D object detectors. Then, if we focus in this case, it seems that the abs-rel metric still corresponds well with 3D object detection rankings, while the others (rms, $\delta < 1.25$) are less informative. 
% Fig 4.6 - PDF
\begin{figure}
    \centering
    \includegraphics[width=1.0\columnwidth]{mde_3od/figures/abs_rel_connections_hr.png}
    \caption{Comparing rankings: abs-rel (MDE) {\vs} $AP_{BEV}-mod$ working at high resolution. In the mid column, we have ordered the MDE models from best (top/1) to worse (bottom/8). Then, we have replicated the mid columns as left (voxel-based detectors, which produce the same ranking) and right (Point R-CNN) columns. Afterwards, we have connected the models in left and right columns to its ranking number according to $AP_{BEV}-mod$. Thus, a perfect correspondence between rankings shows as parallel arrows, and the lower correspondence the more arrows crossing each other.}
    \label{fig:ranking_abs_rel_hr}
\end{figure}

\begin{figure}
    \centering
    \includegraphics[width=1.0\columnwidth]{mde_3od/figures/rms_connections_hr.png}
    \caption{Analogous to \Fig{ranking_abs_rel_hr} using rms metric.}
    \label{fig:ranking_rms_hr}
\end{figure}

\begin{figure}
    \centering
    \includegraphics[width=1.0\columnwidth]{mde_3od/figures/delta1_connections_hr.png}
    \caption{Analogous to \Fig{ranking_abs_rel_hr} using $\delta < 1.25$ metric.}
    \label{fig:ranking_a1_hr}
\end{figure}

\begin{figure}
    \centering
    \includegraphics[width=1.0\columnwidth]{mde_3od/figures/abs_rel_connections_sr.png}
    \caption{Analogous to \Fig{ranking_abs_rel_hr} for low resolution.}
    \label{fig:ranking_abs_rel_sr}
\end{figure}

\begin{figure}
    \centering
    \includegraphics[width=1.0\columnwidth]{mde_3od/figures/rms_connections_sr.png}
    \caption{Analogous to \Fig{ranking_abs_rel_sr} using rms metric.}
    \label{fig:ranking_rms_sr}
\end{figure}

\begin{figure}
    \centering
    \includegraphics[width=1.0\columnwidth]{mde_3od/figures/delta1_connections_sr.png}
    \caption{Analogous to \Fig{ranking_abs_rel_sr} using $\delta < 1.25$ metric.}
    \label{fig:ranking_a1_sr}
\end{figure}
